# Supplementary material for: Uplifting Bandits
Source: arXiv:2206.04091 source file (2022-06-08)
Supplement: Supplementary file 3 [file UpUCB-GapUp-UBL.tex]

% % \subsection{Known Lower Bound on Individual Uplift} \label{sec:part2}


% % \label{sec:part2}
% % Another type of knowledge that can help the learner exploit the structure is a lower bound on individual uplift.
% % This is defined as $\gapUplift>0$ such that for all $\arm\in\arms$ and $\indv\in\va[\variables]$, $\abs{\vav[\meanReward]-\vav[\meanReward][0]}\ge\gapUplift$.
% % Similar assumption were made by \citet{LMT21} to identify which node in the causal graph affects the reward variable.
% % Indeed, this gives us an indicator on how many times we need to take each action in order to identify all its affected variables.

% % Again in this scenario, we derive regret bounds for both when the baseline payoffs are known or not to the learner. 
% % Our algorithms combine UCB, successive elimination \cite{even2006action}, and the idea that the affected variables can be identified after an action is taken sufficiently many times.
% % Our regret bounds feature the ratio $\va[\gapbandit]/\gapUplift$, suggesting that this knowledge is helpful when $\gapUplift$ is relatively large. 
% % We defer details to~\cref{apx:unknown-affected-2}.

% In this second part of~\cref{sec:unknown-affected}, we assume a lower bound on individual uplift is known.
% This means the learner has access to $\gapUplift>0$ satisfying that for all $\arm\in\arms$ and $\indv\in\va[\variables]$, $\abs{\vav[\meanReward]-\vav[\meanReward][0]}\ge\gapUplift$.
% This gives us an indicator on how many times we need to take each action in order to identify all the affected variables. Similar assumption were made by \citet{LMT21} to identify which node in the causal graph affects the reward variable.

% Again in this scenario, we derive regret bounds for both when the baseline payoffs are known or not to the learner. 
% Our algorithms combine UCB, successive elimination \cite{even2006action}, and the idea that the affected variables can be identified after an action is taken sufficiently many times.
% Our regret bounds feature the ratio $\va[\gapbandit]/\gapUplift$, suggesting that this knowledge is helpful when $\gapUplift$ is relatively large. 

% %Our regret bound will feature the ratio $\va[\gapbandit]/\gapUplift$, suggesting that this information is helpful when $\gapUplift$ is relatively large.
% Hereinafter, for any $x,\alpha,\beta\in\R$ with $\alpha\le\beta$, we use $\clip(x,\alpha,\beta)$ to denote the clipping function that restricts $x$ to the interval $[\alpha,\beta]$, \ie $\clip(x,\alpha,\beta)=\max(\alpha,\min(\beta,x))$.

% \subsection{Known Baseline Payoffs}

% As we have seen in \cref{sec:unknown-affected},
% if the baseline payoffs $\va[\meanReward][0]$ are known, we can directly check whether $\vav[\meanReward][0]$ is in the confidence interval.
% Moreover, with the knowledge $\abs{\vav[\meanReward]-\vav[\meanReward][0]}\ge\gapUplift$ for all $\indv\in\va[\variables]$, we deduce that $\va[\variables]$ can be identified correctly with probability $1-2\nVariables\alt{\smallproba}$ after action $\arm$ is taken $\pullcount_0=\ceil{(8/\gapUplift^2)\log(1/\alt{\smallproba})}$ times.
% In fact, let $\vta[\valuev][1],\ldots,\vta[\valuev][\pullcount_0]$ be $\pullcount_0$ i.i.d. realizations of $\va[\valuev]\sim\va[\distribution]$ and $\vtav[\tilde{\meanReward}][\pullcount_0]=(\sum_{\run=1}^{\pullcount_0}\vtav[\valuev])/\pullcount_0$ be the empirical mean of variable $\indv$.
% %Choosing $\varepsilon\in(0,\gapUplift)$ such that $\pullcount_0=(8/(\gapUplift-\varepsilon)^2)\log(1/\alt{\smallproba})$.\footnote{Such $\varepsilon$ exists (and of course, is unique) because $\pullcount_0>(8/\gapUplift^2)\log(2\nVariables/\alt{\smallproba})$.}
% Applying the sub-Gaussian concentration inequality \eqref{eq:sub-Gaussian-concentration} gives
% %
% \begin{equation}
%     \prob\left(\abs{\vtav[\tilde{\meanReward}][\pullcount_0]-\vav[\meanReward]}\ge\frac{\gapUplift}{2}\right)
%     \le2
%     \exp\left(-\frac{\pullcount_0\gapUplift^2}{8}\right)
%     \le 2\alt{\smallproba}.
%     %\frac{\alt{\smallproba}}{\nVariables}.
% \end{equation}
% %
% With a union bound we conclude that with probability at least $1-2\nVariables\alt{\smallproba}$ it holds for all $\indv$ that $\abs{\vtav[\tilde{\meanReward}][\pullcount_0]-\vav[\meanReward]}<\gapUplift/2$.
% We distinguish between the following two situations
% %
% \begin{enumerate}
%     \item $\indv\in\va[\variables]$, then $\displaystyle \abs{\vtav[\tilde{\meanReward}][\pullcount_0]-\vav[\meanReward][0]}\ge\abs{\vav[\meanReward]-\vav[\meanReward][0]}-\abs{\vtav[\tilde{\meanReward}][\pullcount_0]-\vav[\meanReward]}>\gapUplift-\frac{\gapUplift}{2}=\frac{\gapUplift}{2}$.
%     \item $\indv\notin\va[\variables]$, then $\displaystyle \abs{\vtav[\tilde{\meanReward}][\pullcount_0]-\vav[\meanReward][0]}=\abs{\vtav[\tilde{\meanReward}][\pullcount_0]-\vav[\meanReward]}<\frac{\gapUplift}{2}$.
% \end{enumerate}
% %
% This implies that with the choice
% $\va[\setId] = \setdef{\indv\in\variables}{\abs{\vtav[\tilde{\meanReward}][\pullcount_0]-\vav[\meanReward][0]}>\gapUplift/2}$, we have effectively $\prob(\va[\setId]=\va[\variables])\ge1-2\nVariables\alt{\smallproba}$.
% One natural algorithm is to thus first pull each arm $\pullcount_0$ times and run \UpUCB (\cref{algo:UpUCB-BL}) %(from~\cref{subsec:UpUCB-BL})
% in the remaining rounds by regarding $\va[\setId]$ as the variables that action $\arm$ affects.
% A direct computation shows that the regret of this algorithm is in
% $\bigoh(\sum_{\arm\in\arms:\va[\gapbandit]>0}(\va[\gapbandit]/\gapUplift+\va[\nAffected])^2\log\nRuns/\va[\gapbandit])$.
% %$\bigoh(\pullcount_0\sum_{\arm\in\arms}\va[\gapbandit]+(\nArms\nAffected^2)\log\nRuns/\gapbandit)$.

% However, $\pullcount_0$ can be arbitrarily large when $\gapUplift$ gets closer to $0$, and taking an action much fewer times is probably sufficient to deduce that action is not optimal (with high probability).
% We thus propose to implement the above idea in a more flexible manner:
% We run \UpUCB with the uplifting indices $\vta[\UPindexSum]=\sum_{\indv\in\vta[\setId]}(\vtav[\UCBindex]-\vav[\meanReward][0])$, where
% %
% \begin{equation}
%     \notag
%     \vta[\setId] =
%     \begin{cases}
%     \variables & \text{if} ~ \vta[\pullcount]<\pullcount_0,\\
%     \setdef{\indv\in\variables}{\abs{\vtav[\est{\meanReward}][\run][\vt[\arm]]-\vav[\meanReward][0]}>\gapUplift/2} & \text{otherwise}.
%     \end{cases}
% \end{equation}
% %
% %known baseline payoffs by assuming that all the actions affect all the variables.
% %Then, for each arm $\arm$, as long as its pull count exceeds $\pullcount_0$, we switch the index by considering $\va[\setId]$ as the affected set.
% This algorithm is summarized in \cref{algo:UpUCB-GapUp-BL} and has the following regret guarantee.

% \input{Algorithms/UpUCB_GapUp_BL}

% \begin{theorem}
% \label{thm:UpUCB-GapUp-BL-regret}
% Let $\alt{\smallproba}=\smallproba/(2\nArms\nVariables\nRuns)$. Then the regret of \UpUCBDelta (\cref{algo:UpUCB-GapUp-BL}), 
% with probability at least $1-\smallproba$, satisfies:
% %
% \begin{equation}
%     \label{eq:UpUCB-GapUp-BL-regret}
%     \vt[\reg][\nRuns] \le
%     \sum_{\arm\in\arms:\va[\gapbandit]>0}
%     \left(\frac{8\thinspace\clip(\va[\gapbandit]/\gapUplift,\va[\nAffected],\nVariables)^2\log(2\nArms\nVariables\nRuns/\smallproba)}{\va[\gapbandit]}+\va[\gapbandit]\right).
% \end{equation}
% \end{theorem}
% \begin{proof}
% As before, we prove \eqref{eq:UpUCB-GapUp-BL-regret} under the condition that $\event$ defined in \eqref{eq:UCB-L-event} occurs. Recall that we have shown in the proof of \cref{prop:UpUCB-L-BL-regret} that $\prob(\event)\ge1-\smallproba$ with our choice of $\alt{\smallproba}$, so this effectively leads to a high-probability regret bound.

% In the following we assume that $\event$ occurs and show that for any suboptimal action $\arm\in\arms$, it holds
% %
% \begin{equation}
%     \label{eq:UpUCB-GapUp-pullcount-bound}
%     \vta[\pullcount][\nRuns]
%     \le
%     \max\left(
%     \min\left(
%     \frac{8\log(1/\alt{\smallproba})}{\gapUplift^2},
%     \frac{8\nVariables^2\log(1/\alt{\smallproba})}{(\va[\gapbandit])^2}\right), \frac{8(\va[\nAffected])^2\log(1/\alt{\smallproba})}{(\va[\gapbandit])^2}\right)
%     +1.
% \end{equation}
% %
% The inequality \eqref{eq:UpUCB-GapUp-BL-regret} then follows directly from \eqref{eq:regret-decomp-apx} and a rearrangement of the terms.

% We first claim that for any $\arm\in\arms$ if $\vta[\pullcount]\ge\pullcount_0$ then $\vta[\setId]=\va[\variables]$.
% In fact, by the definition of $\pullcount_0$, $\vta[\pullcount]\ge\pullcount_0$ implies that $\vta[\radiusConf]<\gapUplift/2$.
% Therefore, as argued in the text, $\indv\in\vta[\setId]$ if and only if $\indv\in\va[\variables]$.
% Since $\vtav[\UPindex]\ge\vav[\meanUplift]$ for any $\arm$ and $\indv$, this also proves that $\vta[\UPindex]\ge\va[\uplift]$ always holds (we have either $\vta[\setId]=\variables$ or $\vta[\setId]=\va[\variables]$).

% Let $\run\in\intinterval{\nArms+1}{\nRuns}$ be the last time that a suboptimal action $\arm$ is taken so that $\vta[\pullcount][\nRuns]=\vta[\pullcount][\run-1]+1$.
% This indicates $\vta[\UPindexSum]\ge\vta[\UPindexSum][\run][\sol[\arm]]$, and hence $\vta[\UPindexSum]\ge\va[\uplift][\sol[\arm]]$.
% We distinguish between the following two cases:
% %
% \begin{enumerate}[itemsep=2.5pt,topsep=2.5pt,parsep=2.5pt]
%     \item $\vta[\pullcount][\run-1]<\pullcount_0$:
%     Then $\vta[\setId]=\variables$ so $\vta[\UPindexSum]=\sum_{\indv\in\variables}(\vtav[\UCBindex]-\va[\meanReward][0])
%     \le\va[\uplift]+2\nVariables\vta[\radiusConf][\run-1]$, which in turn leads to $\vta[\radiusConf][\run-1]\ge\va[\gapbandit]/(2\nVariables)$, or equivalently $\vta[\pullcount][\run-1]\le8\nVariables^2\log(1/\alt{\smallproba})/(\va[\gapbandit])^2$.
%     \item $\vta[\pullcount][\run-1]\ge\pullcount_0$:
%     Then $\vta[\setId]=\va[\variables]$ so $\vta[\UPindexSum]=\sum_{\indv\in\va[\variables]}(\vtav[\UCBindex]-\va[\meanReward][0])
%     \le\va[\uplift]+2\va[\nAffected]\vta[\radiusConf][\run-1]$, which in turn leads to $\vta[\radiusConf][\run-1]\ge\va[\gapbandit]/(2\va[\nAffected])$, or equivalently $\vta[\pullcount][\run-1]\le8(\va[\nAffected])^2\log(1/\alt{\smallproba})/(\va[\gapbandit])^2$.
% \end{enumerate}
% %
% Since we also have $\vta[\pullcount][\run-1]<\pullcount_0$ in the first case, the above gives
% %
% \begin{equation}
%     \notag
%     \vta[\pullcount][\run-1]
%     \le
%     \max\left(
%     \min\left(
%     \pullcount_0-1,\frac{8\nVariables^2\log(1/\alt{\smallproba})}{(\va[\gapbandit])^2}\right), \frac{8(\va[\nAffected])^2\log(1/\alt{\smallproba})}{(\va[\gapbandit])^2}\right).
% \end{equation}
% %
% Plugging in the definition of $\pullcount_0$ we get immediately \eqref{eq:UpUCB-GapUp-pullcount-bound}.
% \end{proof}

% \cref{thm:UpUCB-GapUp-BL-regret} shows that \cref{algo:UpUCB-GapUp-BL} provides a smooth transition between standard UCB and the strategy that identifies the affected variables of all the actions.
% When $\va[\gapbandit]/\gapUplift\ge\nVariables$, the loss of taking action $\arm$ is so large that UCB prevents it from being taken further even if $\vta[\pullcount]\le\pullcount_0$.
% Otherwise, the affected variables get identified after an action is taken sufficient number of times and the algorithm benefits from this knowledge to improve the estimate of the uplift.
% It is also quite straightforward to combine \cref{algo:UpUCB-L-BL} with \cref{algo:UpUCB-GapUp-BL} when both $\nAffected$ and $\gapUplift$ are known; this results in a regret bound that replaces $\clip(\va[\gapbandit]/\gapUplift,\va[\nAffected],\nVariables)$ by $\clip(\va[\gapbandit]/\gapUplift,\va[\nAffected],\nAffected)$ in \eqref{eq:UpUCB-GapUp-BL-regret}.

% \subsection{Unknown Baseline Payoffs}
% Several additional challenges emerge when we want to adapt the aforementioned strategies to the case where the baseline payoffs are unknown.
% First, without additional assumption, it is impossible to tell whether two arbitrarily close estimates indicate the same effect of two actions on a variable.
% Then, without a proper baseline to compare with, we can never exclude the possibility that all the variables are affected by all the actions.
% We will thus need to make the following much more stringent assumption.

% \begin{assumption}
% \label{asm:gapUplift-ubl}
% The effect of any two actions on a variable differ by at least $\gapUplift$ as long as one of them affects this variable, \ie for all $\arm\in\arms$, $\indv\in\va[\variables]$, and $\alt{\arm}\in\setexclude{\arms}{\{\arm\}}$, it holds $\abs{\vav[\meanReward]-\vav[\meanReward][\alt{\arm}]}\ge\gapUplift$.
% \end{assumption}

% \input{Algorithms/UpUCB_GapUp}

% In other words, $\gapbandit$ is not only a lower bound on individual uplift, but also a lower bound on (individual) effect gap.
% Second, with a UCB-style algorithm, the optimal actions may not be taken sufficiently many times, in which case we can only conservatively assume that they affect all the variables.
% This would incur additional regret in the analysis when $\va[\meanReward][0]$ is unknown. 
% %While this does not pose a problem when $\va[\meanReward][0]$ is known, it can cause extra regret when we apply the \ac{DiffUCB} principle.
% Therefore, we would like to ensure that all the (potentially optimal) actions are taken the same number of times at the point that the affected variables get identified.
% This leads to a two-stage method as described in \cref{algo:UpUCB-GapUp}.

% In the first stage, we perform successive elimination until the uneliminated actions are taken sufficiently many times.
% Here $\vta[\estalt{\reward}][\round]$ is the empirical estimate of the reward associated to action $\arm$ and $\vt[\radiusConf][\round]=\nVariables\sqrt{2\log(1/\alt{\smallproba})/\round}$ is the associated radius of confidence interval.
% %After that, we aggregate variables with close estimates.
% Subsequently, for each variable $\indv\in\variables$ we construct the set
% %
% \begin{equation}
%     \label{eq:setBaseEst}
%     \vv[\setBaseEst]
%     = \setdef{\arm\in\arms}{\exists\thinspace \armalt\in\setexclude{\arms}{\{\arm\}}, \vtav[\intConf][\run_0+1]\intersect\vtav[\intConf][\run_0+1][\armalt]\neq\varnothing},
% \end{equation}
% %
% where $\run_0$ is the number of iterations in the elimination phase and the confidence intervals are defined as in \eqref{eq:UCBs-arm}.
% If \cref{asm:gapUplift-ubl} is verified, then with high probability $\arm\in\vv[\setBaseEst]$ only if $\indv\notin\va[\variables]$.
% Therefore, the observed results from these arms can be used to estimate the baseline payoff of $\indv$.
% The identified variables for action $\arm\in\arms$ are then $\va[\setId]=\setdef{\indv\in\variables}{\arm\notin\vv[\setBaseEst]}$.

% The second stage of the algorithm reuses the idea from \UpUCBwb.
% We define the UCB indices following \eqref{eq:UCBs-arm} for $\arm\in\arms$ and for the baseline estimate we choose among $\vv[\setBaseEst]$ the action that is taken the most frequently whenever this set is non-empty. Otherwise we arbitrarily set it to $0$. That is,
% %
% \begin{equation}
%     \label{eq:UCBs-0-UpUCB-GapUp}
%     \vtav[\UCBindex][\run][0] = \begin{cases}
%     0
%     & \text{if} ~ \vv[\setBaseEst]=\varnothing,
%     \\
%     \vtav[\UCBindex][\run][\vtav[\arm][\run][0]] \text{ where $\vtav[\arm][\run][0]=\argmax_{\arm\in\vv[\setBaseEst]}\vta[\pullcount][\run-1]$} & \text {otherwise}.
%     \end{cases}
% \end{equation}
% %
% The uplifting indices that guide the decision of the algorithm are defined by $\vta[\UPindexSum]=\sum_{\indv\in\vta[\setId]}(\vtav[\UCBindex]-\vtav[\UCBindex][\run][0])$.

% As shown below, the regret of \cref{algo:UpUCB-GapUp} takes roughly the same form as the one in \cref{thm:UpUCB-GapUp-BL-regret}, but as in \cref{thm:UpUCB-regret}, the number of variables that an optimal action affects also plays a crucial role in the regret bound.


% % we form a partition of the remaining arms such that if two arms $\arm, \armalt$ belong to different cells of the partition then the confidence intervals $\vta[\intConf]$ and $\vta[\intConf][\run][\armalt]$ do not overlap.
% % Let us denote by $\vav[\arms]$ the cell that arm $\arm$ belongs to. The aggregated empirical means, pull counts, and UCB indices are defined as:
% % %
% % \begin{equation}
% %     \label{eq:UCBs-gapUplift}
% %     \vtav[\pullcount] = \sum_{\runalt=1}^{\run}\one\{\vt[\arm]\in\vav[\arms]\},
% %     ~~
% %     \vtav[\est{\meanReward}] =
% %     \frac{\sum_{\runalt=1}^{\run}\vtv[\valuev]\one\{\vt[\arm]\in\vav[\arms]\}}{\max(1, \vtav[\pullcount])},
% %     ~~
% %     \vtav[\UCBindex]
% %     = \vtav[\est{\meanReward}]
% %     + \sqrt{\frac{2\log(1/\alt{\smallproba})}{\vtav[\pullcount]}}.
% % \end{equation}
% % %
% % The learner then plays the action with the largest UCB index $\vta[\UCBindex]=\sum_{\indv\in\variables}\vtav[\UCBindex]$.
% % %The whole procedure is described in
% % Notice that if \cref{asm:gapUplift-ubl} is violated, the aggregation of the estimates may incur an additional regret in $\Theta(\nAffected\nRuns\gapUplift)$. 

% % \begin{remark}
% % We do not insist on the use of uplifting index here.
% % Otherwise, another alternative is to compare with some most pulled armed as in \cref{algo:UpUCB-L}.
% % However, we believe aggregating estimates that are close to each other is the most natural thing to do under the assumption that two actions cannot have arbitrarily similar effect on a variable unless they affect the variable in the same way.
% % \end{remark}

% \begin{theorem}
% \label{thm:UpUCB-GapUp-regret}
% Let \cref{asm:gapUplift-ubl} hold and $\alt{\smallproba}=\smallproba/(2\nArms\nVariables\nRuns)$.  Then the regret of \UpUCBDeltawb (\cref{algo:UpUCB-GapUp}), with probability at least $1-\smallproba$, satisfies:
% %
% \begin{equation}
%     \label{eq:UpUCB-GapUp-regret}
%     \vt[\reg][\nRuns] \le
%     \sum_{\arm\in\arms:\va[\gapbandit]>0}
%     \left(\frac{8\thinspace\clip(2\va[\gapbandit]/\gapUplift,\va[\nAffected]+\va[\nAffected][\sol[\arm]],2\nVariables)^2\log(2\nArms\nVariables\nRuns/\smallproba)}{\va[\gapbandit]}+\va[\gapbandit]\right).
% \end{equation}
% \end{theorem}
% \begin{proof}
% We shall again consider the event $\event$ defined in \eqref{eq:UCB-L-event}, which holds with probability $1-\smallproba$ as argued in the proof of \cref{prop:UpUCB-L-BL-regret}. Leveraging the decomposition in \eqref{eq:regret-decomp-apx} it is sufficient to prove that on $\event$ we have
% \begin{equation}
%     \label{eq:UpUCB-GapUp-noBL-pullcount-bound}
%     \vta[\pullcount][\nRuns]
%     \le
%     \max\left(
%     \min\left(
%     \frac{32\log(1/\alt{\smallproba})}{\gapUplift^2},
%     \frac{32\nVariables^2\log(1/\alt{\smallproba})}{(\va[\gapbandit])^2}\right), \frac{8(\va[\nAffected]+\va[\nAffected][\sol[\arm]])^2\log(1/\alt{\smallproba})}{(\va[\gapbandit])^2}\right)
%     +1.
% \end{equation}
% %
% We assume $\event$ happens in the rest of the proof.

% Let us first focus on the elimination phase, notice that event $\event$ implies $\abs{\vta[\estalt{\reward}][\round]-\va[\reward]}<\vt[\radiusConf][\round]$ for every $\arm\in\vt[\arms][\round]$.
% % We define the event
% % %
% % \begin{equation}
% %     \notag
% %     \event_1 =
% %     \left\{\forall\round\in\oneto{\pullcount_0},
% %     ~\forall\arm\in\arms,
% %     ~ \abs{\vta[\estalt{\reward}][\round]-\va[\reward]}<\nVariables\sqrt{\frac{2\log(1/\alt{\smallproba})}{\round}}\right\}
% % \end{equation}
% % %
% % Following the proof of \cref{lem:concentration-mean-a} and a union bound over $\arm\in\arms$, we know that $\prob(\event_1)\ge1-2\nArms\pullcount_0\alt{\smallproba}$.
% In this case, the optimal actions never get eliminated.
% In fact, if $\sol[\arm]\in\vt[\arms][\round]$, then for all $\arm\in\vt[\arms][\round]$ it holds that
% %
% \begin{equation}
%     \notag
%     \vta[\estalt{\reward}][\round][\sol[\arm]]
%     +2\vt[\radiusConf][\round]
%     \ge
%     \va[\reward][\sol[\arm]]+\vt[\radiusConf][\round]
%     \ge
%     \va[\reward][\arm]+\vt[\radiusConf][\round]
%     \ge \vta[\estalt{\reward}][\round][\arm],
% \end{equation}
% %
% As a consequence, we also have $\sol[\arm]\in\vt[\arms][\round+1]$ and we conclude by the principle of induction.
% With this we further deduce that all action
% $\arm$ with $\va[\gapbandit]\ge4\vt[\radiusConf][\round]$ gets eliminated
% %\nVariables\sqrt{2\log(1/\alt{\smallproba})/\round}$ 
% after it is taken at most $\round$ times.
% %must be eliminated at the latest in round $\round$. 
% To see this, notice that for such action we have
% %
% \begin{equation}
%     \notag
%     \vta[\estalt{\reward}][\round]+2\vt[\radiusConf][\round]
%     < \va[\reward]+3\vt[\radiusConf][\round]
%     = \va[\reward][\sol[\arm]]-\va[\gapbandit]+3\vt[\radiusConf][\round]
%     < \vta[\estalt{\reward}][\round][\sol[\arm]]
%     -\va[\gapbandit]+4\vt[\radiusConf][\round]
%     \le \vta[\estalt{\reward}][\round][\sol[\arm]].
% \end{equation}
% %
% Therefore, for all $\run$ in phase \rom{1} of the algorithm, it is true that
% %
% \begin{equation}
%     \label{eq:UpUCB-GapUp-noBL-pullcount-bound-I}
%     \vta[\pullcount]\le
%     \min\left(
%     \left\lceil\frac{32\log(1/\alt{\smallproba})}{\gapUplift^2}\right\rceil,
%     \left\lceil\frac{32\nVariables^2\log(1/\alt{\smallproba})}{(\va[\gapbandit])^2}\right\rceil
%     \right).
% \end{equation}
% %
% This suggests that inequality \eqref{eq:UpUCB-GapUp-noBL-pullcount-bound} holds if the algorithm terminates in the elimination phase.

% Otherwise, the algorithm constructs $\vv[\setBase]$'s, $\va[\setId]$'s, and switches to the \textsc{UpUCB} phase.
% Let us denote by $\vv[\setBase]=\setdef{\arm\in\arms}{\indv\notin\va[\variables]}$ the set of actions that do not affect variable $\indv$
% and let $\arms_{\text{res}}=\vt[\arms][\pullcount_0+1]$ be the actions that remain after phase \rom{1}.
% %$\pullcount_0=\ceil{(32/\gapUplift^2)\log(1/\alt{\smallproba})}$ be the number of times that the uneliminated arms are pulled in the first phase.
% We argue that the sets $\vv[\setBaseEst]$ are constructed such that when $\event$ occurs,
% \begin{enumerate}[\textup(\itshape i\textup)]
%     \item $\vv[\setBaseEst]\subseteq\vv[\setBase]$.
%     \item  If there exist $\arm,\armalt\in\arms_{\text{res}}\intersect\vv[\setBase]$ such that $\arm\neq\armalt$ then we also have $\arm,\armalt\in\vv[\setBaseEst]$.
% \end{enumerate}
% %
% The second point is proved by observing that under $\event$ we must have $\vav[\meanReward][0]\in\vtav[\intConf][\run_0+1]\intersect\vtav[\intConf][\run_0+1][\armalt]$ if $\arm,\armalt\in\arms_{\text{res}}\intersect\vv[\setBase]$.
% To show the first point, notice that after the elimination phase, each of the action in $\arms_{\text{res}}$ is taken exactly $\ceil{(32/\gapUplift^2)\log(1/\alt{\smallproba})}$ times and thus $\vta[\radiusConf][\run_0]\le\gapUplift/4$.
% By \cref{asm:gapUplift-ubl}, if $\arm\notin\vv[\setBase]$, then for all $\armalt\in\setexclude{\arms_{\text{res}}}{\{\arm\}}$ we have $\abs{\vav[\meanReward]-\vav[\meanReward][\alt{\arm}]}\ge\gapUplift$, which along with the definition of $\event$ implies $\vtav[\intConf][\run_0+1]\intersect\vtav[\intConf][\run_0+1][\armalt]=\varnothing$, and therefore $\arm\notin\vv[\setBaseEst]$.

% The rest of the proof follows closely that of \cref{thm:UpUCB-regret}.
% Suppose that a suboptimal action $\arm$ is taken at round $\run$ during phase \rom{2} of the algorithm.
% This means $\vta[\UPindexSum]\ge\vta[\UPindexSum][\run][\sol[\arm]]$ (recall that $\sol[\arm]\in\arms_{\text{res}}$ since $\event$ happens), \ie
% %
% \begin{equation}
%     \notag
%     \sum_{\indv\in\va[\setId]}(\vtav[\UCBindex][\run]-\vtav[\UCBindex][\run][0])
%     \ge
%     \sum_{\indv\in\va[\setId][\sol[\arm]]}
%     (\vtav[\UCBindex][\run][\sol[\arm]]-\vtav[\UCBindex][\run][0]).
% \end{equation}
% %
% Rearranging the terms we get 
% %
% \begin{equation}
%     \notag
%     \sum_{\indv\in\va[\setId]}\vtav[\UCBindex][\run]
%     +\sum_{\indv\in\setexclude{\va[\setId][\sol[\arm]]}{\va[\setId]}}
%     \vtav[\UCBindex][\run][0]
%     \ge
%     \sum_{\indv\in\va[\setId][\sol[\arm]]}
%     \vtav[\UCBindex][\run][\sol[\arm]]
%     +\sum_{\indv\in\setexclude{\va[\setId]}{\va[\setId][\sol[\arm]]}}
%     \vtav[\UCBindex][\run][0].
% \end{equation}
% %
% If $\indv\in\setexclude{\va[\setId][\sol[\arm]]}{\va[\setId]}$ then $\arm\in\vv[\setBaseEst]$.
% In particular, $\vv[\setBaseEst]\neq\varnothing$ so $\armalt=\vtav[\arm][\run][0]=\argmax_{\tilde{\arm}\in\vv[\setBaseEst]}\vta[\pullcount][\run-1][\tilde{\arm}]$ is well-defined and $\vtav[\UCBindex][\run][0]=\vtav[\UCBindex][\run][\armalt]$.
% With $\vv[\setBaseEst]\subseteq\vv[\setBase]$ we know that $\vav[\meanReward][\armalt]=\vav[\meanReward][0]$ and accordingly $\abs{\vtav[\meanReward][\run-1][\armalt]-\vav[\meanReward][0]}\le\vta[\radiusConf][\run-1][\armalt]$ by the fact that $\event$ happens.
% This shows $\vtav[\UCBindex][\run][0]\ge\vav[\meanReward][0]$.
% Moreover, $\vta[\pullcount][\run][\armalt]\ge\vta[\pullcount]$ by the choice of $\armalt$; hence, $\vtav[\UCBindex][\run][0]\le\vav[\meanReward][0]+2\vta[\radiusConf][\run-1][\armalt]\le\vav[\meanReward][0]+2\vta[\radiusConf][\run-1]$.
% The same argument applies to $\indv\in\setexclude{\va[\setId]}{\va[\setId][\sol[\arm]]}$, and the UCB indices of $\arm$ and $\sol[\arm]$ can be bounded from above and below as in previous proofs.
% In summary, we obtain
% %
% \begin{equation}
%     \notag
%     \sum_{\indv\in\va[\setId]}(\vav[\meanReward]+2\vta[\radiusConf][\run-1])
%     +\sum_{\indv\in\setexclude{\va[\setId][\sol[\arm]]}{\va[\setId]}}
%     (\vav[\meanReward][0]+2\vta[\radiusConf][\run-1])
%     \ge
%     \sum_{\indv\in\va[\setId][\sol[\arm]]}
%     \vav[\meanReward][\sol[\arm]]
%     +\sum_{\indv\in\setexclude{\va[\setId]}{\va[\setId][\sol[\arm]]}}
%     \vav[\meanReward][0].
% \end{equation}
% %
% Equivalently,
% %
% \begin{equation}
%     \label{eq:UpUCB-GapUp-radConf-larger-than}
%     2\card\left(\va[\setId]\union\va[\setId][\sol[\arm]]\right)\vta[\radiusConf][\run-1]
%     \ge
%     \sum_{\indv\in\va[\setId]\union\va[\setId][\sol[\arm]]}\vav[\meanReward][\sol[\arm]]
%     -\sum_{\indv\in\va[\setId]\union\va[\setId][\sol[\arm]]}\vav[\meanReward].
% \end{equation}
% %
% To conclude, we claim that
% %
% \begin{equation}
%     \label{eq:VV-equal}
%     \va[\setId]\union\va[\setId][\sol[\arm]]=\va[\variables]\union\va[\variables][\sol[\arm]].
% \end{equation}
% %
% Let us first show $\va[\variables]\subseteq\va[\setId]\subseteq\va[\variables]\union\va[\variables][\sol[\arm]]$.
% The first inclusion is a consequence of $\vv[\setBaseEst]\subseteq\vv[\setBase]$:
% %
% \begin{equation}
%     \notag
%     \indv\in\va[\variables] \implies
%     \arm\notin\vv[\setBase] \implies
%     \arm\not\in\vv[\setBaseEst] \implies
%     \indv\in\va[\setId].
% \end{equation}
% %
% As for the second inclusion we prove it's contrapositive:
% %
% \begin{equation}
%     \notag
%     \indv\notin\va[\variables]\union\va[\variables][\sol[\arm]] \implies
%     \arm,\sol[\arm]\in\arms_{\text{res}}\intersect\vv[\setBase] \implies
%     \arm,\sol[\arm]\in\vv[\setBaseEst] \implies
%     \indv\notin\va[\setId]
% \end{equation}
% %
% Notice that the second implication holds because $\arm$ is suboptimal and in particular $\arm\neq\sol[\arm]$.
% The inclusion $\va[\variables][\sol[\arm]]\subseteq\va[\setId][\sol[\arm]]\subseteq\va[\variables]\union\va[\variables][\sol[\arm]]$ can be proved in a similar way, and combining these results gives \eqref{eq:VV-equal}.
% Therefore, the \acl{RHS} of \eqref{eq:UpUCB-GapUp-radConf-larger-than} is exactly $\va[\gapbandit]$ while the \acl{LHS} of \eqref{eq:UpUCB-GapUp-radConf-larger-than} is bounded from above by $2(\va[\nAffected]+\va[\nAffected][\sol[\arm]])\vta[\radiusConf][\run-1]$.
% In consequence,
% %
% \begin{equation}
%     \notag
%     \vta[\pullcount][\run-1]
%     \le \frac{8(\va[\nAffected]+\va[\nAffected][\sol[\arm]])^2\log(1/\alt{\smallproba})}{(\va[\gapbandit])^2}.
% \end{equation}
% %
% Therefore, any suboptimal action that gets taken in the \textsc{UpUCB} phase satisfies
% %
% \begin{equation}
%     \notag
%     \vta[\pullcount][\nRuns]
%     \le \frac{8(\va[\nAffected]+\va[\nAffected][\sol[\arm]])^2\log(1/\alt{\smallproba})}{(\va[\gapbandit])^2}+1.
% \end{equation}
% %
% On the other hand, if an suboptimal action is not taken in the \textsc{UpUCB} phase then \eqref{eq:UpUCB-GapUp-noBL-pullcount-bound-I} applies, so in either case \eqref{eq:UpUCB-GapUp-noBL-pullcount-bound} is verified, which concludes the proof.
% \end{proof}

% \vspace{0.4em}
% \begin{remark}
% A natural candidate for $\vtav[\UCBindex][\run][0]$ is the one that uses aggregated information as in \eqref{eq:mean-estimate-0}.
% The problem of this choice is that how we aggregate the observations collected in the first phase are only determined at the end of the the phase, while this choice itself depends on these observations.
% Mathematically, this prevents us from defining a suitable martingale difference sequence for which we establish concentration bound.
% An easy fix is to only aggregate observations from the second phase, while the use of the observations from the first phase should be limited to those coming from just one arm.
% %in $\vv[\setBaseEst]$.
% \end{remark}
