# Supplementary material for: Uplifting Bandits
Source: arXiv:2206.04091 source file (2022-06-08)
Supplement: Supplementary file 12 [file Concentration-deprecated.tex]

In this section, we formally describe the probability model of the $\nArms$-arm uplifting bandit problem that we build upon for proving the regret upper bounds, before deriving several concentration results that are used throughout our analyses.

Our upper-bound analyses are based on the stack-feedback model.
That is, we have a collection of independent random vectors $(\vta[\valuev][\round])_{\arm\in\arms,\round\in\oneto{\nRuns}}$ such that the law of $\vta[\valuev][\round]$ is $\va[\distribution]$.
Each $(\vta[\valuev][\round])_{\round\in\oneto{\nRuns}}$ forms a stack, and when the learner chooses action $\arm$, they receives the vector from the top of the stack. In other words, the value of $\vta[\valuev][\round]$ is observed when the learner pulls $\arm$ for the $\round$-th time.
By abuse of notation, we will also use $\vta[\valuev][\round]$ to denote the value of the random variable (evaluated at some $\sample\in\samples$ with $\samples$ being the underlying probability space).
In most of our algorithms, we are interested in either of the following estimates
%
\begin{equation}
    \notag
    \vtav[\estalt{\meanReward}][\round]=\frac{\sum_{\runalt=1}^{\round}\vtav[\valuev][\runalt]}{\round},
    ~~~~~~
    \vtav[\est{\meanReward}][\run][0] =
    \frac{\sum_{\runalt=1}^{\run}\vtav[\valuev][\runalt][\vt[\arm][\runalt]]\one\{\indv\notin\va[\variables][\vt[\arm]]\}}{\max(1, \vtav[\pullcount][\run][0])}.
\end{equation}
%
Despite the apparent similarity between these two quantities, the key distinction is that the denominator of $\vtav[\estalt{\meanReward}][\round]$ is a constant while the denominator of $\vtav[\est{\meanReward}][\run][0]$ is also a random variable.
Therefore, deriving a concentration bound for the later will require a more delicate treatment.
We first state a concentration inequality for $\vtav[\estalt{\meanReward}][\round]$.
%
\begin{lemma}
\label{lem:iid-concentration}
Let $\smallproba\in(0,1)$. It holds
%
\begin{equation}
    \notag
    \prob\left(\abs{\vtav[\estalt{\meanReward}][\round]-\vav[\meanReward]}\ge\sqrt{\frac{2\log(1/\smallproba)}{\round}}\right)
    \le 2\smallproba.
\end{equation}
\end{lemma}
\begin{proof}
This is immediate from \eqref{eq:subgaussian-concentration} and the fact that $\vtav[\estalt{\meanReward}][\round]$ is $(1/\sqrt{\round})$-subgaussian.
\end{proof}
%
\cref{lem:iid-concentration} is sufficient for the analysis whenever $\vtav[\est{\meanReward}]$ is defined as in \eqref{eq:mean-estimate-a}.
In fact, in this case $\vtav[\est{\meanReward}]=\vtav[\estalt{\meanReward}][\vta[\pullcount]]$ as long as $\vta[\pullcount]\ge1$.
Therefore, if $\abs{\vtav[\estalt{\meanReward}][\round]-\vav[\meanReward]}\le\sqrt{2\log(1/\alt{\smallproba})/\round}$ for all relevant $\arm$ and $\indv$ we have indeed the desired concentration result.

For the more challenging case where an indicator of the probability event is also involved in the estimator, we will leverage on tools from martingale theory.
Let us first introduce a concentration inequality for martingale difference sequence based on \cite[Lem. 2]{BDHK+08} and \cite[Th. 1.2A]{Victor99}.

\begin{lemma}%[{{\cite[Lem. 2]{BDHK+08}}}]
\label{lem:DLP-ineq}
Let $(\vt[\filter][\runalt])_{\runalt=0}^{\run}$ be a filtration and $(\vt[\rv][\runalt])_{\runalt=1}^{\run}$ be a $(\vt[\filter][\runalt])$-adapted martingale difference sequence.
Suppose that there exists $\rvb>0$ such that $\exof{\vt[\rv][\runalt]^2\given{\vt[\filter][\runalt-1]}}\le\rvb^2$ and that the following conditional Bernstein condition is verified for all $\runalt\in\oneto{\run}$ and $\probmoment\ge2$,
\begin{equation}
    \notag
    \exof{\abs{\vt[\rv][\runalt]}^{\probmoment}\given{\vt[\filter][\runalt-1]}} \le \frac{\probmoment!}{2}\rvb^{\probmoment-2}\exof{\vt[\rv][\runalt]^2\given{\vt[\filter][\runalt-1]}}.
\end{equation}
Then, for any $\smallproba\in(0,1/e)$, it holds
%
\begin{equation}
    \notag
    \prob\left(\sum_{\runalt=1}^{\run}\vt[\rv][\runalt]
    \ge 2\max(2\noisedev,2\rvb\sqrt{\log(1/\smallproba)})\sqrt{\log(1/\smallproba)}
    \right) \le \max(\log_2(\run),1)\frac{\smallproba}{2},
\end{equation}
where $\noisedev=\sqrt{\sum_{\runalt=1}^{\run}\exof{\vt[\rv][\runalt]^2\given{\vt[\filter][\runalt-1]}}}$ is the square root of the sum of the conditional variances of $\vt[\rv][\runalt]$'s.
\end{lemma}
\begin{proof}
The proof of \cite[Lem. 2]{BDHK+08} essentially applies.
We just need to replace the use of Freedman’s inequality by the use of de la Peña's inequality \cite[Th. 1.2A]{Victor99} and define $\alpha_0=2\rvb\sqrt{\log(1/\smallproba)}$.
Also notice with this choice of $\alpha_0$ the condition $\smallproba<1/e$ guarantees $\alpha_0\ge2$ so $\ell\ge\log_2{\sqrt{\run}}-1$ already ensures $2^{\ell}\alpha_0\ge\rvb\sqrt{\run}$.
\end{proof}

In the following, $(\vt[\filter])_{\run}$ will represent the natural filtration associated to $(\vt[\valuev], \vt[\arm][\run+1])_{\run}$ such that both $\vt[\valuev]$ and $\vt[\arm][\run+1]$ are $\vt[\filter]$-measurable.

\begin{lemma}
\label{lem:indicator-concentration}
Let $(\eventalt)_{\runalt=1}^{\run}$ be a sequence of events such that $\vt[\eventalt][\runalt]\in\vt[\filter][\runalt-1]$.
We consider
\begin{equation}
    \notag
    \vta[\pullcount][\run][\eventalt] = \sum_{\runalt=1}^{\run}\one\{\vt[\eventalt][\runalt]\},
    ~~~~~
    \vtav[\est{\meanReward}][\run][\eventalt] =
    \frac{\sum_{\runalt=1}^{\run}\vtav[\valuev][\runalt][\vt[\arm][\runalt]]
    \one\{\vt[\eventalt][\runalt]\}}
    {\max(1, \vta[\pullcount][\run][\eventalt])}.
\end{equation}
%
Suppose that all the noise variables $\vav[\snoise]$ satisfy the Bernstein condition \eqref{eq:Bernstein} with $\noisedev=1$ and have their variance bounded by $1$ (this is automatically verified if the noises are $1$-subgaussian).
Then, we have the following concentration bound for $\vtav[\est{\meanReward}][\run][\eventalt]$
%
\begin{equation}
    \label{eq:indicator-estimate-concentration}
    \prob
    \left(
    \left|\vtav[\est{\meanReward}][\run][\eventalt] - \frac{\sum_{\runalt=1}^{\run}\vav[\meanReward][\vt[\arm][\runalt]]\one\{\vt[\eventalt][\runalt]\}}{ \max(1,\vta[\pullcount][\run][\eventalt])}\right|
    \ge
    4\sqrt{\frac{\log((\log(\run)/\log(2))\smallproba)}
    {\max(1,\vta[\pullcount][\run][\eventalt])}}
    + \frac{4\log((\log(\run)/\log(2))\smallproba)}
    {\max(1,\vta[\pullcount][\run][\eventalt])}
    \right)
    \le \smallproba
\end{equation}
\end{lemma}
\begin{proof}
Let $\vtav[\snoise][\runalt][\vt[\arm][\runalt]]=\vtav[\valuev][\runalt][\vt[\arm][\runalt]]-\vav[\meanReward][\vt[\arm][\runalt]]$.
We apply \cref{lem:DLP-ineq} with $\vt[\rv][\runalt]\subs\vtav[\snoise][\runalt][\vt[\arm][\runalt]]\one\{\vt[\eventalt][\runalt]\}$ and $\rvb\subs 1$.
The two conditions that involve $\rvb$ in \cref{lem:DLP-ineq} are indeed verified because
$\ex_{\runalt-1}[\abs{\vtav[\snoise][\runalt][\vt[\arm][\runalt]]\one\{\vt[\eventalt][\runalt]\}}^{\probmoment}]=\ex[\abs{\vav[\snoise][\vt[\arm][\runalt]]}^{\probmoment}]\one\{\vt[\eventalt][\runalt]\}$ for all $\probmoment\in\R$.
The equality with $\probmoment=2$ also shows that $\ex_{\runalt-1}[\vt[\rv][\runalt]^2]\le\one\{\vt[\eventalt][\runalt]\}$ and thus $\sum_{\runalt=1}^{\run}\ex_{\runalt-1}[\vt[\rv][\runalt]^2]\le\vta[\pullcount][\run][\eventalt]$.
\cref{lem:DLP-ineq} then ensures that for all $\alt{\smallproba}\in(0,1/e)$, it holds
%
\begin{equation}
    \notag
    \prob\left(\sum_{\runalt=1}^{\run}
    (\vtav[\valuev][\runalt][\vt[\arm][\runalt]]-\vav[\meanReward][\vt[\arm][\runalt]])\one\{\vt[\eventalt][\runalt]\}
    \ge 4\sqrt{\vta[\pullcount][\run][\eventalt]\log(1/\alt{\smallproba})}
    + 4\log(1/\alt{\smallproba})
    \right) \le \frac{\log(\run)\alt{\smallproba}}{2\log(2)}.
    %\le \log(\run)\alt{\smallproba}.
\end{equation}
%
Applying the same procedure to $\vt[\rv][\runalt]\subs-\vtav[\snoise][\runalt][\vt[\arm][\runalt]]\one\{\vt[\eventalt][\runalt]\}$ and using a union bound we get
%
\begin{equation}
    \notag
    \prob\left(\sum_{\runalt=1}^{\run}
    \abs{(\vtav[\valuev][\runalt][\vt[\arm][\runalt]]-\vav[\meanReward][\vt[\arm][\runalt]])\one\{\vt[\eventalt][\runalt]\}}
    \ge 4\sqrt{\vta[\pullcount][\run][\eventalt]\log(1/\alt{\smallproba})}
    + 4\log(1/\alt{\smallproba})
    \right) \le  \frac{\log(\run)\alt{\smallproba}}{\log(2)}.
\end{equation}
%
We obtain \eqref{eq:indicator-estimate-concentration} by dividing the inequality in $\prob$ by $\max(1,\vta[\pullcount][\run][\eventalt])$ and choose $\alt{\smallproba}=(\log(2)/\log(\run))\smallproba<1/e$.
\end{proof}

\begin{lemma}
Suppose that $\vav[\snoise][0]$ satisfies the Bernstein condition \eqref{eq:Bernstein} with $\noisedev=1$ and its variance is bounded by $1$.
Let $\smallproba\in(0,1/e)$. It holds
\begin{equation}
    \notag
    \prob
    \left(
    \abs{\vtav[\est{\meanReward}][\run][0] - \vav[\meanReward][0]}
    \ge
    4\sqrt{\frac{\log(2\run/\alt{\smallproba})}{\vtav[\pullcount][\run][0]}}
    + \frac{4\log(2\run/\alt{\smallproba})}{\vtav[\pullcount][\run][0]}
    \right)
    \le \smallproba.
\end{equation}
\end{lemma}
\begin{proof}
The result is immediate from \cref{lem:indicator-concentration} with the choice $\vt[\eventalt][\runalt]=\{\indv\notin\va[\variables][\runalt]\}$.
We also use the inequality $\log(\run)/(\log(2)\max(1,\vtav[\pullcount][\run][0]))\le2\run/\vtav[\pullcount][\run][0]$ and the fact that $\vav[\meanReward][\vt[\arm][\runalt]]\one\{\indv\notin\va[\variables][\runalt]\}=\vav[\meanReward][0]\one\{\indv\notin\va[\variables][\runalt]\}$.
\end{proof}
